# Supplementary material for: Probing cage relaxation in concentrated protein solutions by XPCS
Source: arXiv:2203.12695 source file (2022-03-23)
Supplement: Supplementary file 1 [file main_v3_SI.pdf]

# Supplementary information
# Probing cage relaxation in concentrated protein solutions by XPCS

Yuriy Chushkin[†,1,*] Alessandro Gulotta,[2,†] Felix Roosen-Runge,[3,2,†]
Antara Pal,[2] Anna Stradner,[2,4] and Peter Schurtenberger[2,4,‡]

[1]*ESRF, The European Synchrotron, 71 Avenue des Martyrs, CS40220, 38043 Grenoble Cedex 9, France*
[2]*Division for Physical Chemistry, Lund University, Naturvetarvägen 14, 22100 Lund, Sweden*
[3]*Department of Biomedical Sciences and Biofilms-Research Center for Biointerfaces (BRCB), Faculty of Health and Society, Malmö University, Sweden*
[4]*Lund Institute of advanced Neutron and X-ray Science LINXS, Lund University, Lund, Sweden*

(Dated: March 23, 2022)

## STRUCTURE ANALYSIS

The typical scattered intensity obtained by SAXS from a concentrated $\alpha$-crystallin solution is shown in Fig. S1 (a). The structure factor $S(q)$ was obtained by fitting the measured curve with the polydisperse hard-sphere model [1]. From the fit the position of the peak $q^*$ and its height $S(q^*)$ were extracted and their dependence on the dose and the dose rate was analyzed (see Fig. 1 in the main text and Fig. S1 (c)).

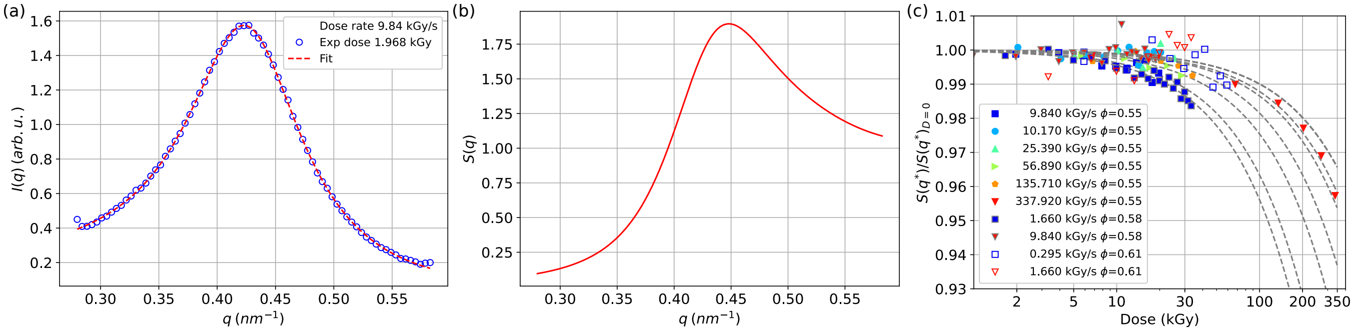


Fig. S 1. (a) Measured scattered intensity of the concentrated $\alpha$-crystallin solution at volume fraction $\phi$=0.55, where the red dashed line is a fit using a polydisperse hard-sphere model. (b) The structure factor $S(q)$ obtained from the fit of the data in (a). (c) Evolution of the relative height of the structure factor $S(q^*)$ with dose for different volume fractions and dose rates used. The dashed line is a fit with an exponential decay to the data.

## DYNAMICS ANALYSIS

The observed slow drift of the peak position $q^*$ with the dose (time) shown in Fig. 1 in the main text can result in the decorrelation of the measured intensity correlation function. Such a decorrelation can be modeled by an exponential decay of the following form: $\exp(-(\upsilon/\Delta q \cdot \tau)^2)$, where $\upsilon = (q^*(0) - q^*(t))/t$ is the velocity of the drift in reciprocal space, and $\Delta q$ is the pixel size in reciprocal space. The calculated decays are show in Fig. S2 with the dashed dotted lines. The color corresponds to the dose rate of the experimental data.

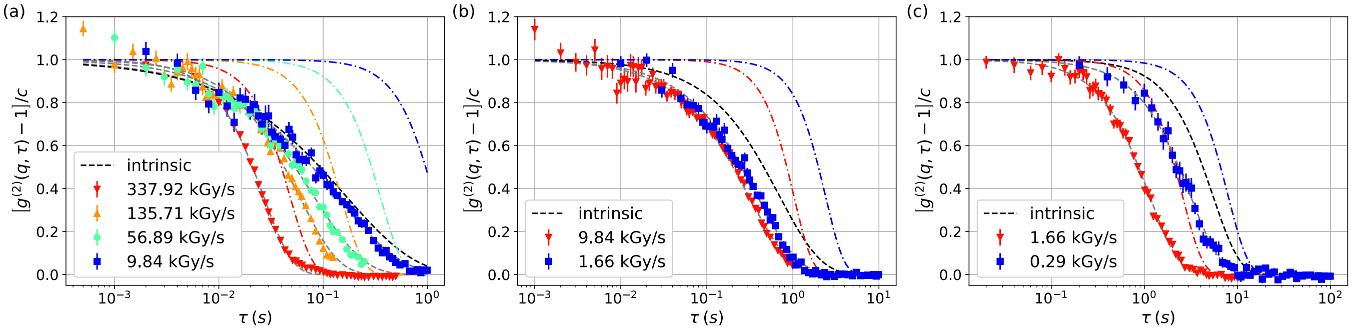


Fig. S 2. Measured normalized intensity correlation functions at different dose rates and volume fractions (a) $\phi$=0.55, (b) $\phi$=0.58 and (c) $\phi$=0.61. Dashed lines are fits with KWW expression. Black dashed line is expected intrinsic relaxation decay. Dashed dotted lines are decorrelation related to the shift of $q^*$ for dose rates used.

Figure S3 shows two examples of the measured two-time correlation function [2]:

$$C(t_1, t_2) = \frac{\langle I_p(t_1) I_p(t_2)\rangle_p}{\langle I_p(t_1)\rangle_p \langle I_p(t_2)\rangle_p}, \quad (1)$$

where $I_p(t)$ is the intensity in pixel $p$ at time $t$ and $\langle\rangle_p$ is the average over pixels belonging to the same range of a scattering vector magnitude. The two-time correlation functions show the evolution of the relaxation time (width of the red diagonal band) with time. The time dependent $g^{(2)}(q, \tau)$ was calculated by averaging $C(t_1, t_2)$ over the relevant times.

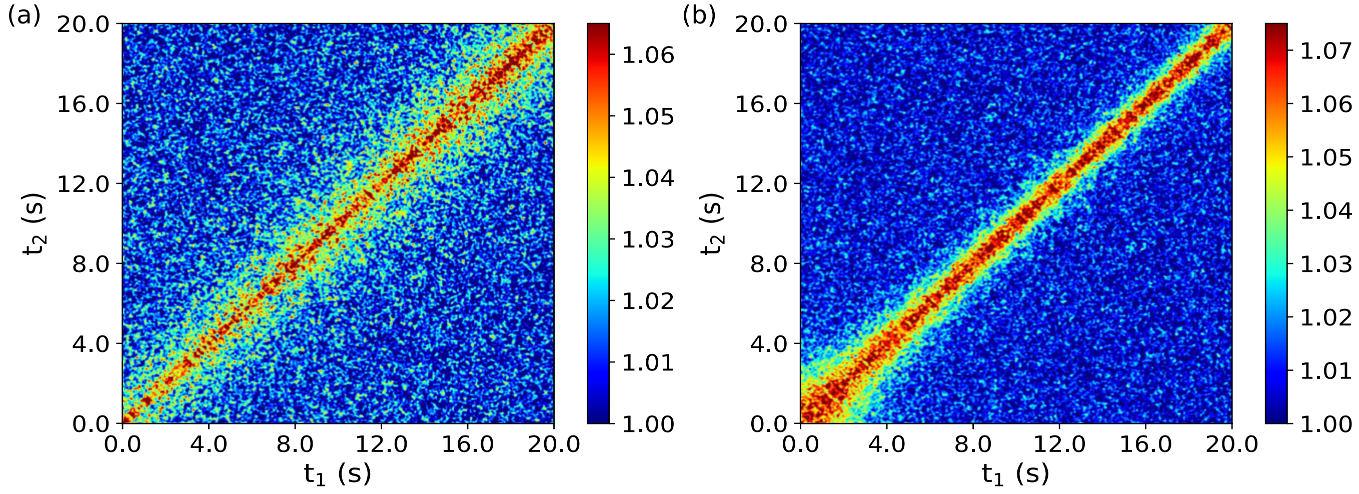


Fig. S 3. Two-time correlation function of the sample at (a) $\phi = 0.55$ using 9.84 kGy/s dose rate and (b) $\phi = 0.61$ using 1.66 kGy/s dose rate.

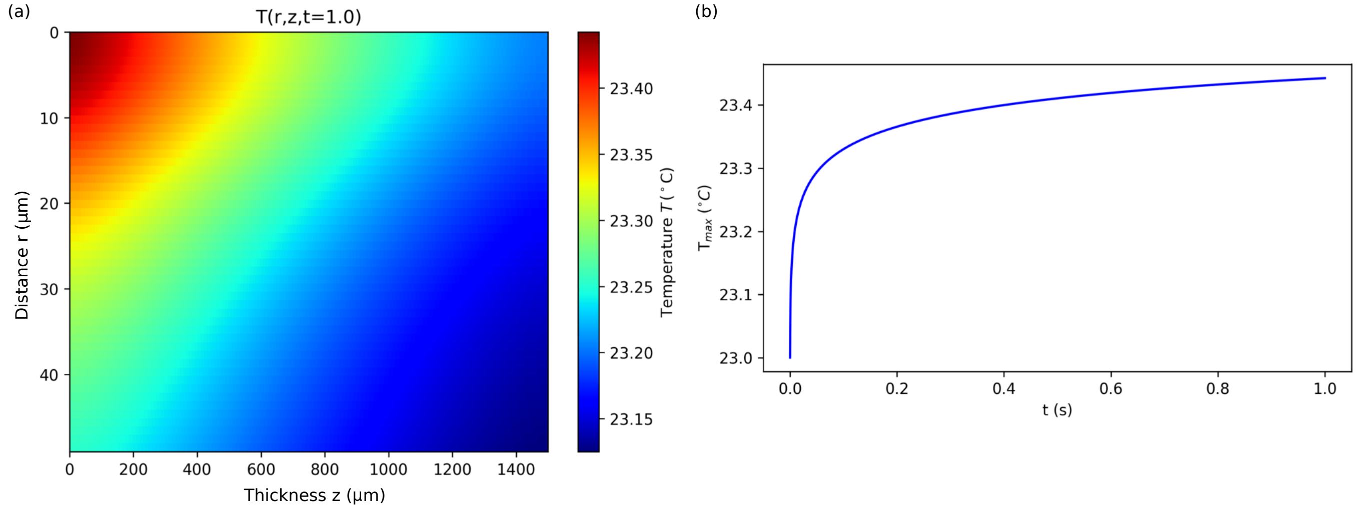


Fig. S 4. (a) Temperature distribution after 1 second exposure under the strongest dose rate condition of 337.92 kGy/s. Only the area of 50 $\mu m$ around the beam center is shown. (b) Temporal evolution of the maximum sample temperature $T_{max}$.

## THERMAL ANALYSIS

The thermal effect of the X-ray beam illumination was calculated using a finite difference method [3]. We assumed that the energy of all absorbed photons was transformed to heat. The heat generation inside a sample (we used waters' thermal properties) was modeled using a Gaussian beam profile with a FWHM of 20 $\mu m$, and taking into account the X-ray absorption profile along the capillary thickness z of 1.5 mm. The calculations were done in a cylindrical coordinate system neglecting the heat evacuation through the capillary walls, therefore the estimated temperature is expected to be higher than the actual one. The sample temperature evolution with time at the maximum dose rate used (337.92 kGy/s) is shown in Fig. S4. The estimated maximum sample temperature increase is ∼0.44 degrees. At lower dose rates the temperature increase is obviously smaller.

---

* chushkin@esrf.fr; These three authors contributed equally
† These three authors contributed equally

‡ peter.schurtenberger@fkem1.lu.se

[1] A. Vrij, The Journal of Chemical Physics **71**, 3267 (1979), https://doi.org/10.1063/1.438756.
[2] M. Sutton, K. Laaziri, F. Livet, and F. Bley, Opt. Express **11**, 2268 (2003).
[3] Ozisik, Orlande, Colaco, and Cotta, *Finite Difference Methods in Heat Transfer, Second Edition* (CRC Press, 2017).
